# Supplementary material for: Nonequilibrium transport in density-modulated phases of the second Landau level
Source: arXiv:1412.4702 source file (2015-06-27)
Supplement: Supplementary file 1 [file SI_v3.pdf]

# Nonequilibrium transport in density-modulated phases of the second Landau level
# -
# Supplementary Information

S. Baer*,[1] C. Rössler,[1] S. Hennel,[1] H.C. Overweg,[1] T. Ihn,[1] K. Ensslin,[1] C. Reichl,[1] and W. Wegscheider[1]

[1]*Solid State Physics Laboratory, ETH Zürich, 8093 Zürich, Switzerland*

(Dated: June 27, 2015)

**RIQH phase diagram for wafer A**

Similar to Fig. 2, we can extract a phase diagram for wafer A from the measurement shown in Fig. S.1.a. The corresponding critical Hall voltages are shown in Fig. S.1.b,c for the different RIQH states.

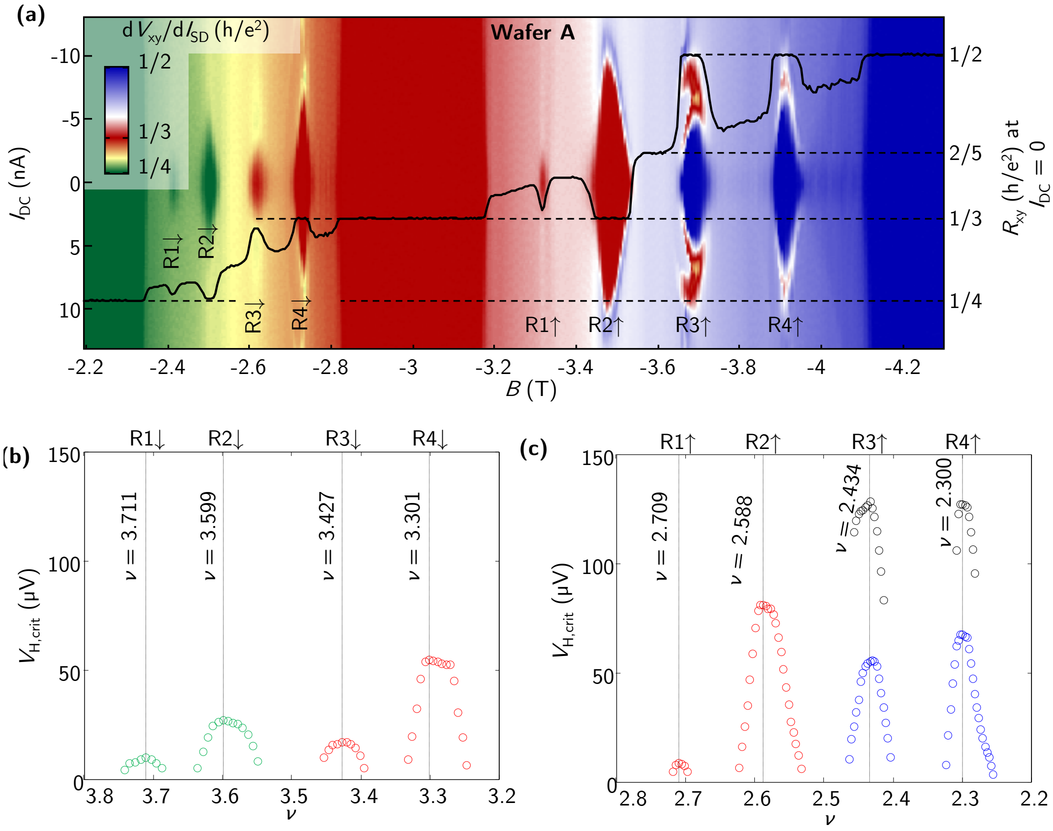


FIG. S.1: **a**: Differential Hall resistance measured with wafer A. **b**: Critical Hall voltage for the breakdown of the RIQH states with $R_{xy} = 1/4 \times h/e^2$ (green) and $R_{xy} = 1/3 \times h/e^2$ (red) and for the transition to an isotropic background (black). **c**: Critical Hall voltage for the breakdown of the RIQH states with $R_{xy} = 1/3 \times h/e^2$ (red) and $R_{xy} = 1/2 \times h/e^2$ (blue) and for the transition to an isotropic background (black).
